# Supplementary material for: Melting points of water models: Current situation
Source: arXiv:2401.11812 source file (2024-01-22)
Supplement: Supplementary file 1 [file supplementary.pdf]

# Supplementary material

## Melting points of water models: Current situation

S. Blazquez<sup>1</sup> and C. Vega<sup>1</sup>

<sup>1</sup>*Departamento Química Física I, Facultad de Ciencias Químicas,  
Universidad Complutense de Madrid, 28040 Madrid, Spain*

We present now the results of the simulations of each model studied in this work.

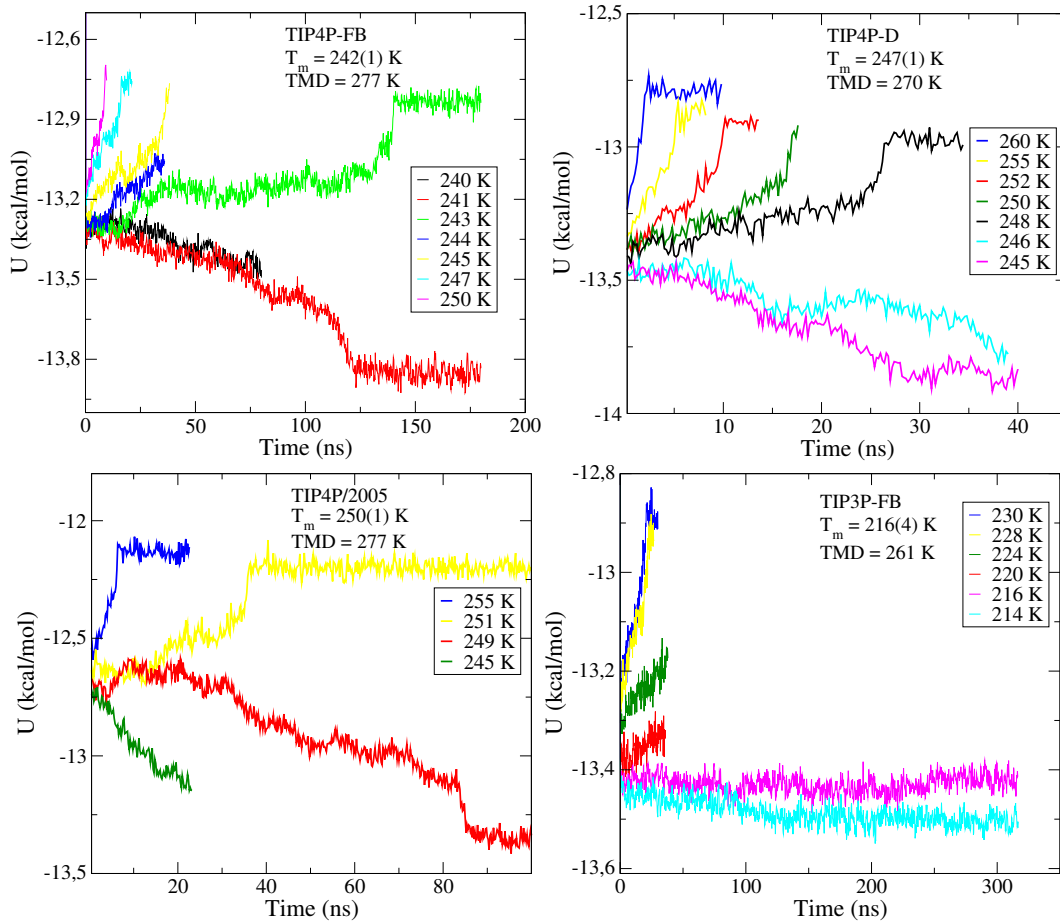

FIG. 1. Evolution of the potential energy as a function of time for the NpT runs of the different models at 1 bar and different temperatures: a)TIP4P-FB b)TIP4P-D c)TIP4P/2005 d)TIP3P-FB

As we have explained in the note, the method to determine the melting temperature consists in the study of the evolution of potential energy of the system (coexistence ice-water) in function of time for different temperatures. The idea is that when the potential

energy goes down the ice is growing and when the potential energy is going up the ice melts. Thus, we can estimate the melting temperature between the highest temperature at which the ice grows and the lowest temperature at which the ice melts. The melting point can also be evaluated by free energy methods (i.e by computing the chemical potential of water in the solid and in the liquid phase). In this case one must add an additional contribution (Pauling entropy which is  $-RT\ln(3/2)$  for ice Ih) to the chemical potential of the solid to account for the many possible configurations compatible with the Bernal-Fowler rules responsible for the proton disorder of ice Ih, since free energy methods compute the chemical potential of a particular proton-disordered configuration. When using direct coexistence even though one is using a particular proton-disordered configuration for the solid the correct melting point is obtained. Notice that the fluid-solid interface is dynamic and in the growth-melting process many different proton disordered configurations are sampled at the interface.<sup>1</sup>

In Figure 1 we show the evolution of the potential energy in function of time for different temperatures and water models. As can be seen in Figure 1a), for the TIP4P-FB model at all temperatures above 243 K (including it) the ice melts. And at all temperatures below 241 K the ice grows. Thus, we can conclude that the melting temperature for the TIP4P-FB model is  $T_m = 242(1)$  K. Following the same procedure, we estimate that the melting temperature of TIP4P-D force field is  $T_m = 247(1)$  K. To establish a proper comparison we have recalculated the melting temperature of TIP4P/2005 using exactly the same system size and conditions that were used for the other water models considered in this work, obtaining  $T_m = 250(1)$  K. Finally, we present also the results for a 3-site model, the TIP3P-FB. In this case it is more difficult to evaluate its melting temperature because of the slow dynamics at such low temperatures. Nevertheless we estimate the melting temperature in  $T_m = 216(4)$  K

Let us now present the results for the TIP5P model. This is the first time that we revisit the melting point of this force field. In figure 2 we can see the ice melts at 275 K. On the contrary, ice grows for 270, 272 and 273 K. Thus, we conclude that the melting point of TIP5P force field is  $274(2)$  K. In 2006 we estimated the melting point of this model in  $272(3)$  K<sup>2</sup>. The system used in that work was smaller (870 water molecules in total) and the simulations lengths were also shorter (about 10 ns). In this work we obtain a value slightly higher than in that work, improving the previous results obtained almost 20 years ago.

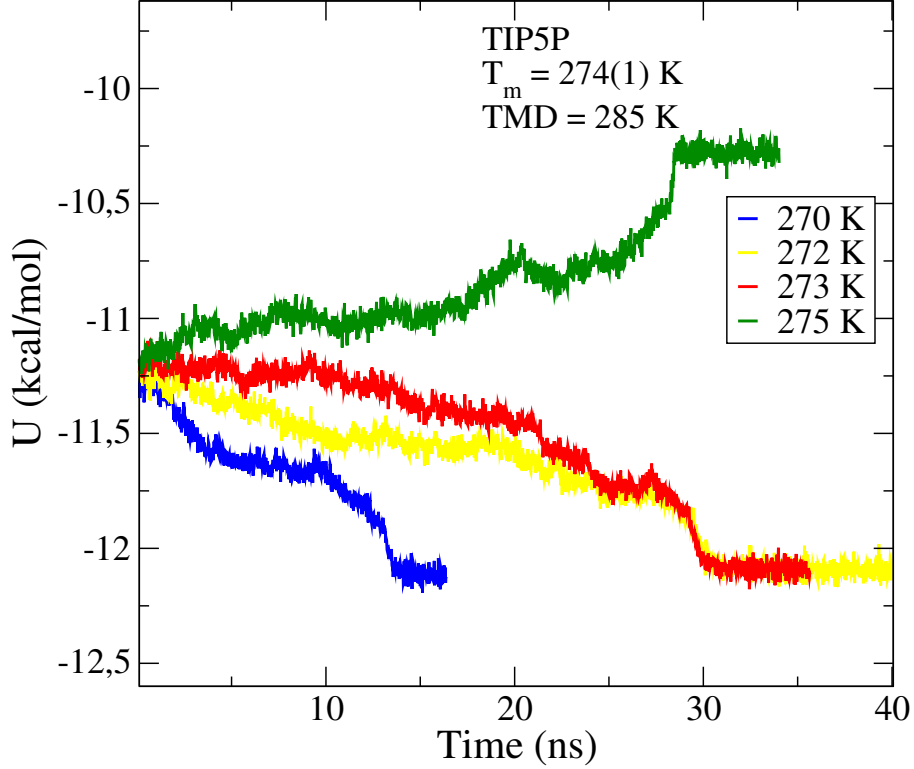

FIG. 2. Evolution of the potential energy as a function of time for the NpT runs of the TIP5P model at 1 bar and different temperatures.

We have also plotted the energies of the three four center models in the same graph. In Figure 3 we can see that the time required to grow for the ice depends on the model. It is pretty clear that the TIP4P-D water model grows faster than the TIP4P-2005 and this one grows faster than the TIP4P-FB.

As a final point we will present now the melting enthalpies of the models studied in this work. We have also calculated the melting enthalpy of the OPC<sup>3</sup> and TIP4P/Ice<sup>4</sup> water models. The melting point of this water model was calculated accurately by Onufriev and coworkers.<sup>5</sup> However, they did not provide the melting enthalpy of the model. To calculate this property we have run two independent NpT simulations. The first one was a 100 ns simulation of a cubic box containing 555 molecules of liquid water. The second one was a 20 ns simulation of a box containing 2000 molecules of ice. We run both simulations at

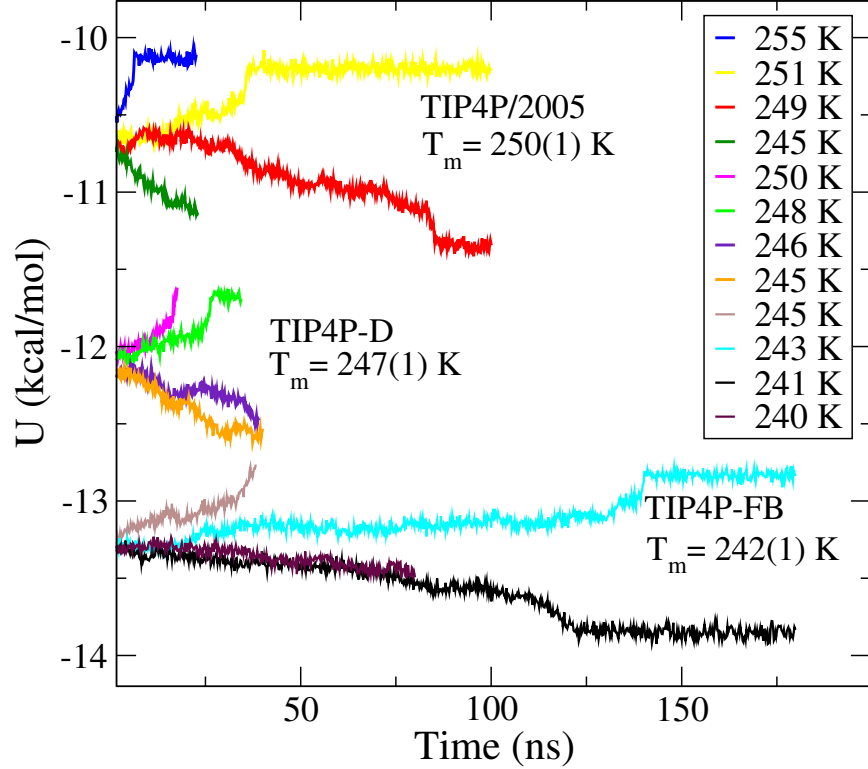

FIG. 3. Evolution of the potential energy as a function of time for the NpT runs of the different models at 1 bar and different temperatures in only one plot. The energies for the TIP4P-D and TIP4P-2005 have been shifted 1.3 and 2.0 kcal/mol respectively.

1 bar and at the melting temperature of the model. We used a cutoff of 1.0 nm for both simulations. The difference between the enthalpy of liquid water and that of ice Ih is the melting enthalpy of the model. In Table I we present the melting enthalpies of the different models.

As it can be seen in Fig. 4a) There is no model which reproduces the experimental melting enthalpy. The 3-site models greatly underestimated the experimental results. 5-site models overestimate it. And 4-site models also underestimate the experimental enthalpy (although they work better than 3-site force fields). In Fig. 4b) it is clear that the TIP4P/2005 is the only force field able to simultaneously reproduce the experimental density of liquid water and ice. Finally we show also the difference between the densities of the liquid and the ice (i. e.  $\Delta\rho = \rho_{liq} - \rho_{ice}$ ). We can see that only TIP4P/Ice and TIP4P/2005 are able to reproduce

TABLE I. Melting enthalpies and ice and liquid water densities at the melting temperature of the different water models calculated in this work.

| Model             | $\Delta H_m$ | $\rho_{liquid}$   | $\rho_{ice}$      |
|-------------------|--------------|-------------------|-------------------|
|                   | kcal/mol     | kg/m <sup>3</sup> | kg/m <sup>3</sup> |
| <b>Expt.</b>      | 1.44         | 999               | 917               |
| <b>TIP3P-FB</b>   | 0.63         | 991               | 946               |
| <b>TIP4P/2005</b> | 1.13         | 994               | 920               |
| <b>TIP4P/Ice</b>  | 1.22         | 987               | 906               |
| <b>OPC</b>        | 1.07         | 995               | 895               |
| <b>TIP4P-FB</b>   | 0.99         | 987               | 926               |
| <b>TIP4P-D</b>    | 1.11         | 995               | 888               |
| <b>TIP5P</b>      | 1.78         | 986               | 967               |

correctly this difference.

- 
- <sup>1</sup> C. Vega, E. Sanz, E. G. Noya, and J. L. F. Abascal, J. Phys. Condens. Matter **20**, 153101 (2008).
- <sup>2</sup> R. G. Fernandez, J. L. F. Abascal, and C. Vega, J. Chem. Phys. **124**, 144506 (2006).
- <sup>3</sup> S. Izadi, R. Anandakrishnan, and A. V. Onufriev, **5**, 3863 (2014).
- <sup>4</sup> J. L. F. Abascal, E. Sanz, R. García Fernández, and C. Vega, J. Chem. Phys. **122**, 234511 (2005).
- <sup>5</sup> Y. Xiong, P. S. Shabane, and A. V. Onufriev, ACS Omega **5**, 25087 (2020).

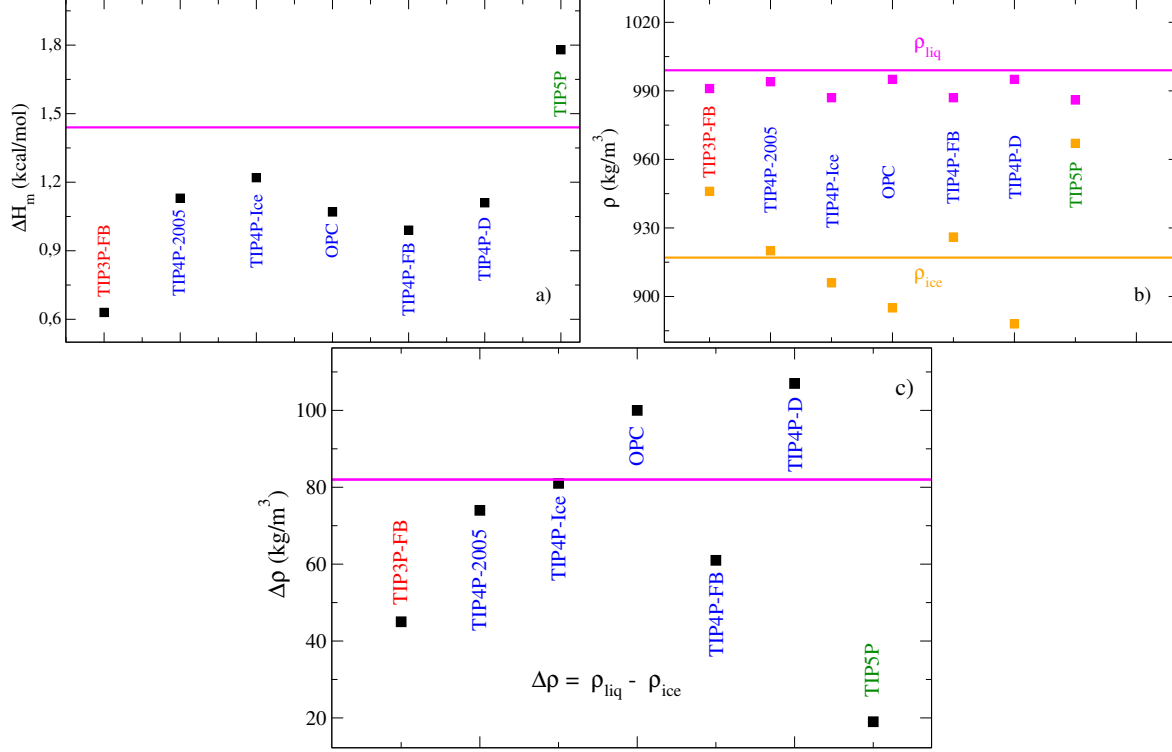

FIG. 4. a) Melting enthalpies of each model studied at its melting temperature. Solid magenta line is the experimental enthalpy. Black squares are the simulation results for each model. b) Ice and liquid water densities at the melting temperature of the different water models calculated in this work. Solid magenta and orange lines are the experimental densities of liquid and ice respectively. The results of the densities of each model are plotted as squares: Magenta for the liquid densities and orange for the ice densities. c) Difference between the density of the liquid and the density of the ice. Magenta solid line is the experimental difference and the black squares are the differences for each force field calculated in this work.
